# Supplementary material for: Spatio-Temporal Modeling of Users' Check-ins in Location-Based Social Networks
Source: arXiv:1611.07710 source file (2017-04-10)
Supplement: Supplementary file 1 [file 08-Appendix.tex]

%% Appendix
%\appendix
%\section*{APPENDIX}
%\setcounter{section}{1}
%In this appendix, we measure
%the channel switching time of Micaz [CROSSBOW] sensor devices.
%In our experiments, one mote alternatingly switches between Channels
%11 and 12. Every time after the node switches to a channel, it sends
%out a packet immediately and then changes to a new channel as soon
%as the transmission is finished. We measure the
%number of packets the test mote can send in 10 seconds, denoted as
%$N_{1}$. In contrast, we also measure the same value of the test
%mote without switching channels, denoted as $N_{2}$. We calculate
%the channel-switching time $s$ as
%\begin{eqnarray}%
%s=\frac{10}{N_{1}}-\frac{10}{N_{2}}. \nonumber
%\end{eqnarray}%
%By repeating the experiments 100 times, we get the average
%channel-switching time of Micaz motes: 24.3$\mu$s.
%
%\appendixhead{ZHOU}
%
%
%\section{This is an example of Appendix section head}
%
%Channel-switching time is measured as the time length it takes for
%motes to successfully switch from one channel to another. This
%parameter impacts the maximum network throughput, because motes
%cannot receive or send any packet during this period of time, and it
%also affects the efficiency of toggle snooping in MMSN, where motes
%need to sense through channels rapidly.
%
%By repeating experiments 100 times, we get the average
%channel-switching time of Micaz motes: 24.3 $\mu$s. We then conduct
%the same experiments with different Micaz motes, as well as
%experiments with the transmitter switching from Channel 11 to other
%channels. In both scenarios, the channel-switching time does not have
%obvious changes. (In our experiments, all values are in the range of
%23.6 $\mu$s to 24.9 $\mu$s.)
%
%\section{Appendix section head}
%
%The primary consumer of energy in WSNs is idle listening. The key to
%reduce idle listening is executing low duty-cycle on nodes. Two
%primary approaches are considered in controlling duty-cycles in the
%MAC layer.
